# Supplementary material for: Boiling in Nanopores through Localized Joule Heating: Transition between Nucleate and Film Boiling
Source: arXiv:2207.09799 ancillary file (2022-07-20)
Supplement: Supplementary file 1 [file SI_EDITED.pdf]

# Supplemental Material for "Boiling in Nanopores through Localized Joule Heating: Transition between Nucleate and Film Boiling"

Soumyadeep Paul, Wei-Lun Hsu, Yusuke Ito, and Hirofumi Daiguji*

*Department of Mechanical Engineering, The University of Tokyo, Hongo, Tokyo, Japan*

E-mail: daiguji@thml.t.u-tokyo.ac.jp

## S1. SEM images of cylindrical nanopores

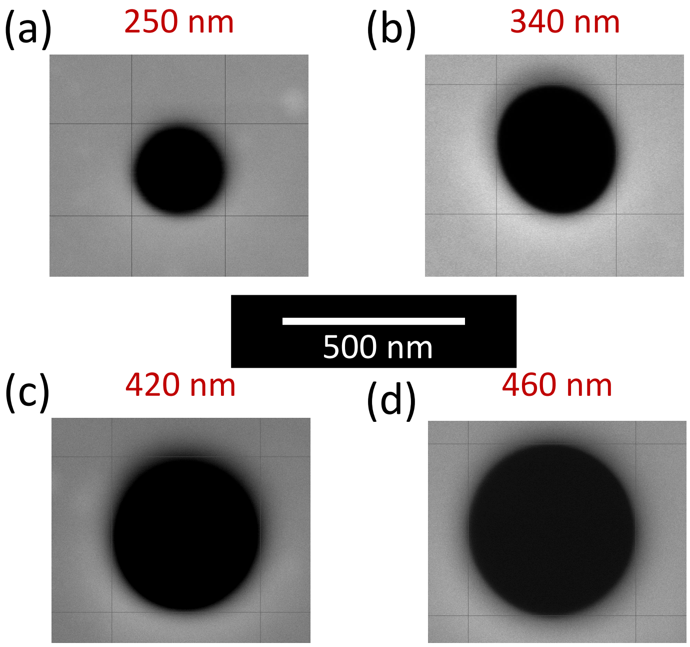


Figure S1: SEM images of the four nanopores used in the present study.

## S2. Hydrophone positioning

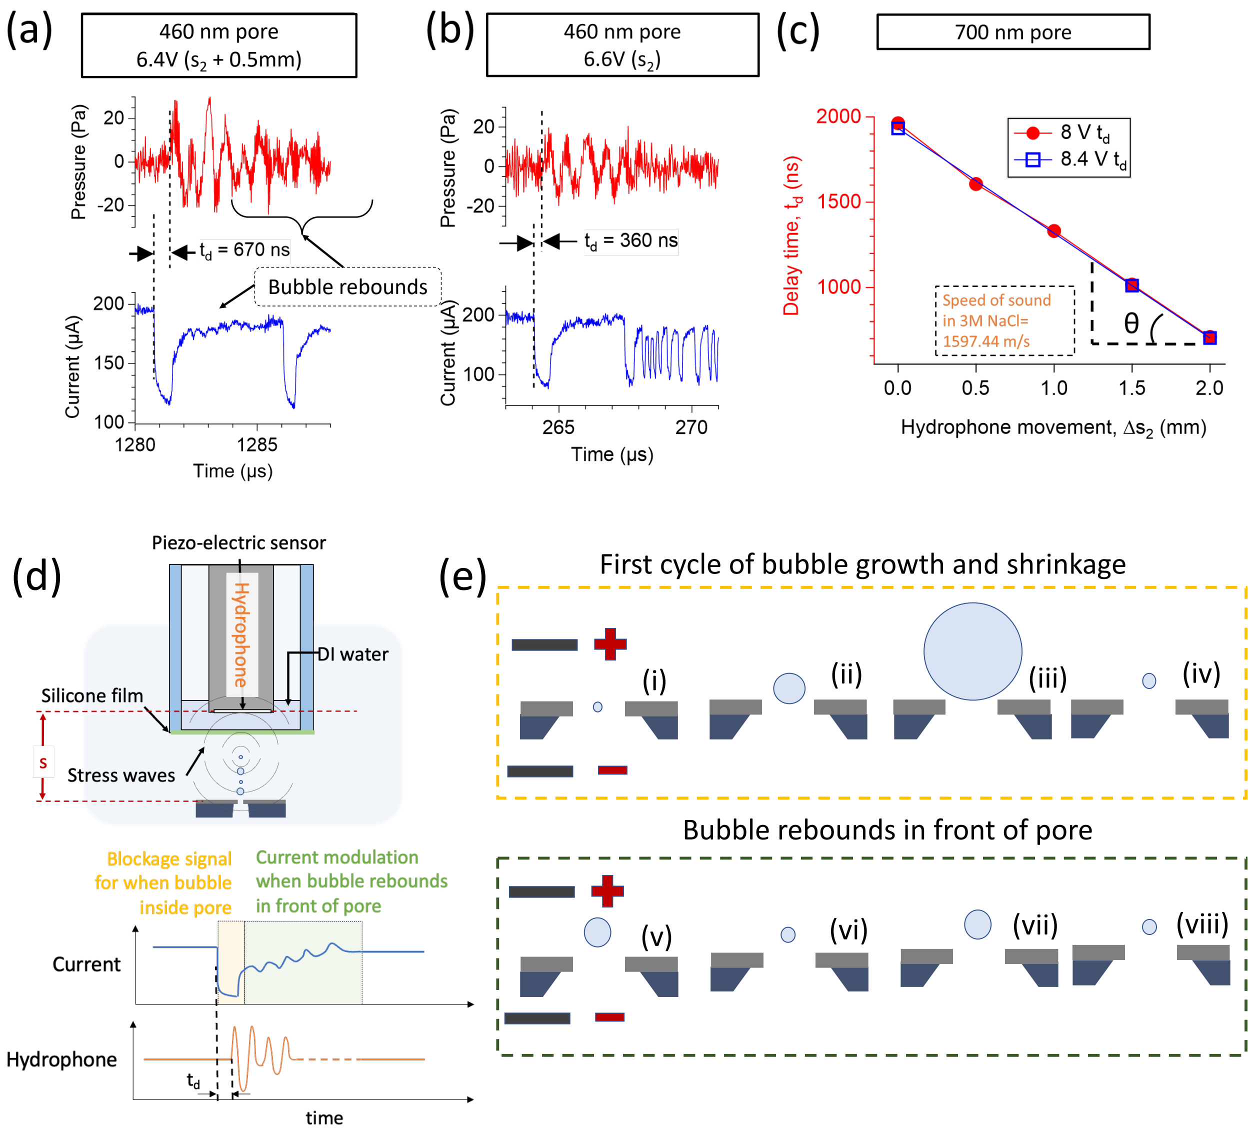


Figure S2: (a) and (b) Current and pressure signals of homogeneous bubble nucleation inside a 460 nm pore at 6.3 V and 6.6 V, respectively. (c) Linear variation of delay time with hydrophone movement, using which the speed of sound in 3M NaCl is calculated. (d) Schematic explanation of nanopore bubble stress waves and the reason for the delay time. (e) Schematic explanation of homogeneous bubble growth and collapse during the first cycle (top) and subsequent rebounding behavior near the pore entrance (bottom), causing current waviness.

The clearance distance is lower by 0.5 mm in Fig. S2(a) compared with S2(b). As a result, the delay time $t_d$ between current dip and pressure rise increases by 310 ns. According to

this calculation, the speed of sound in 3M NaCl becomes 1613 m/s. This is comparable to the results of the previous experiments done for a 700 nm pore [Fig. S2(c)], where a linear relation between $t_\mathrm{d}$ and hydrophone vertical movement $\Delta s_2$ was found and the slope of the line gave the speed of sound as1597.44 m/s. This analysis also shows that the hydrophone is electrically insulated and the signals represent only the effect of stress waves. Also, it can be seen that the amplitude of the pressure signal is higher for a smaller clearance but lower voltage [Fig. S2(a)], indicating that the pressure signal recorded by the hydrophone is not influenced by ionic current in the electrolyte.

## S3. Torus bubble dynamics

### Torus bubble geometric properties

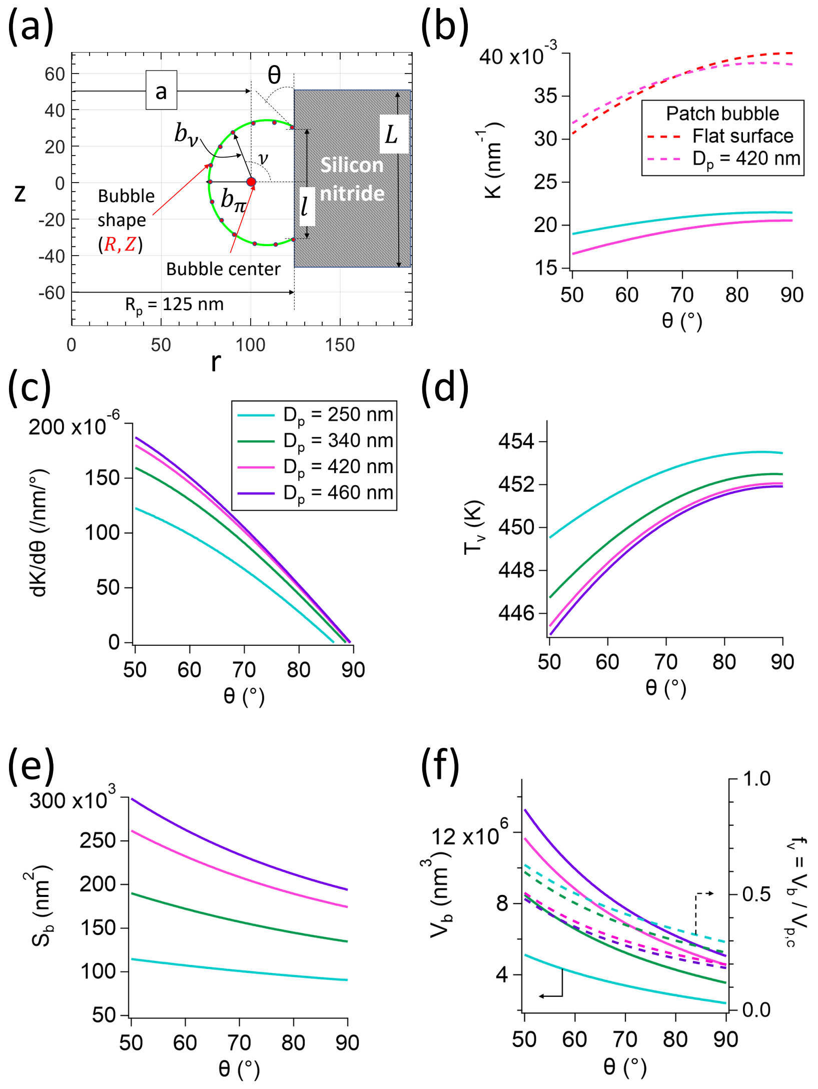


Figure S3: (a) Parameters controlling the torus bubble shape on the pore surface. We assume that the torus bubble is pinned, which means that $l = L$. (b) Comparison of the curvature of the torus bubble (solid lines) with that of patch bubbles (dashed lines) for the same $L$. It can be seen that compared with patch bubbles, torus bubbles having the same $\theta$ and $L$ have 50% lower curvature. Also, the $K$ variation with $\theta$ is flatter for torus bubbles in general, and more so for smaller pore diameter. This is because the bubble is convex, whereas the pore surface is concave. (c) Gradient of curvature with contact angle variation. The color coding for different pore diameters shown here is used in the other plots as well. (d) Torus bubble temperature, according to Laplace's equation. (e) Bubble liquid/vapor surface area. (f) Bubble volume (solid lines) and fraction of pore volume exclusion $f_v$ (dashed lines).

**Torus bubble stability properties**

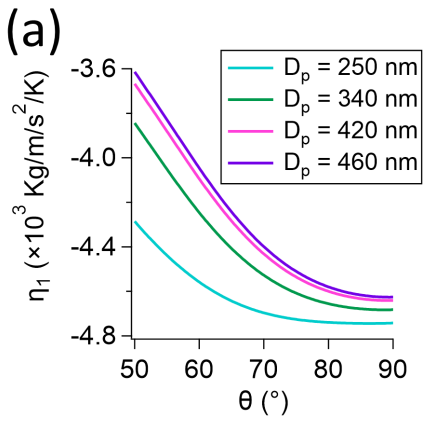


Figure S4: Stability parameters of torus bubble: (a) $\eta_1$; (b) $\eta_2$.

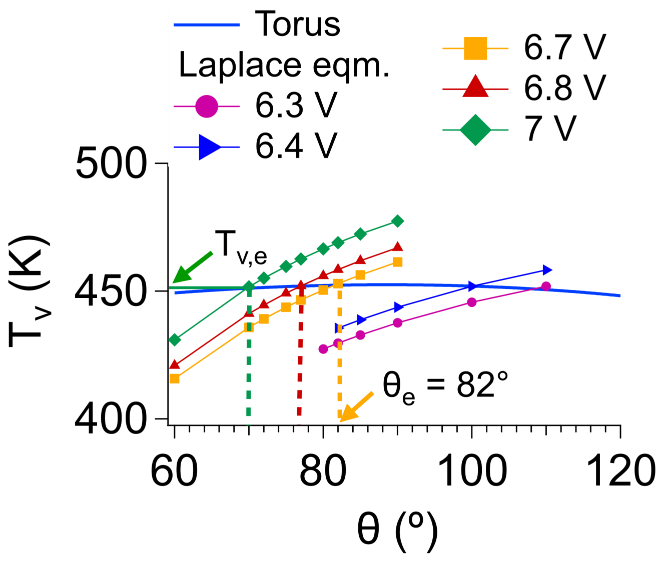


Figure S5: Equilibrium temperature of torus bubble inside 340 nm pore.

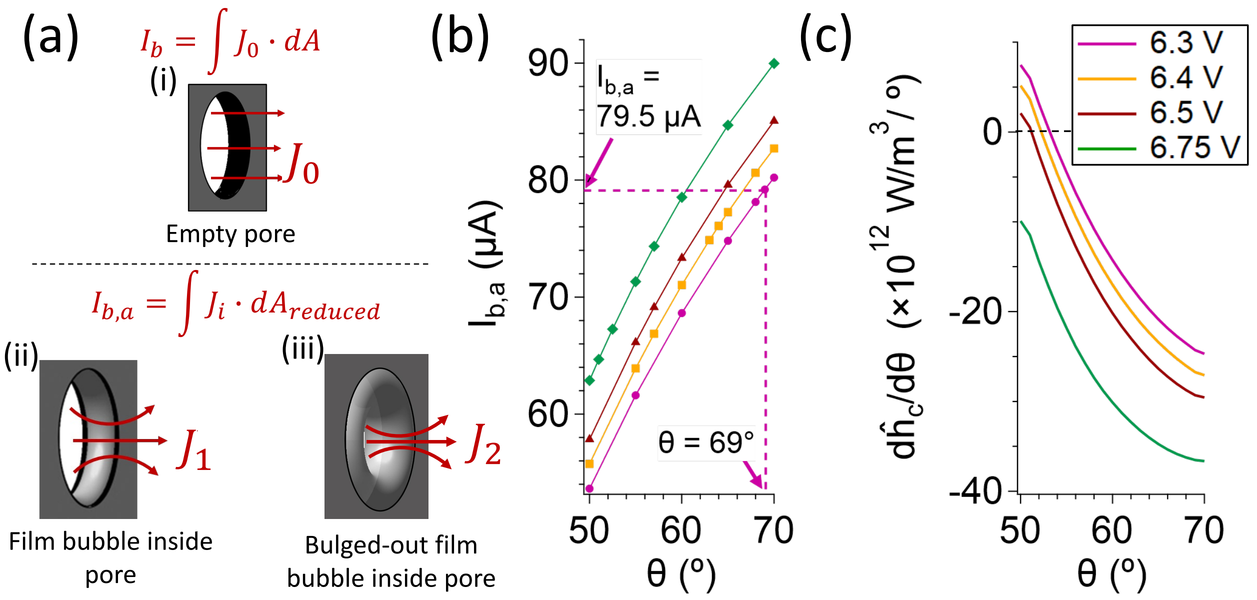


Figure S6: (a) Schematic representation of the torus bubble position and how the ionic flux $J$ is affected. As the effective pore cross-sectional area decreases from $A = \pi R_\mathrm{p}^2$ to $A_\mathrm{reduced} = \pi r_\mathrm{v}^2$ owing to torus bubble formation, the nanopore current decreases from $I_\mathrm{b}$ to $I_\mathrm{b,a}$. Now, as the torus bubble bulges out in a pinned state, $\mathbf{J} = \sigma\mathbf{E}$ will increase as the average electric field inside the pore, $|\mathbf{E}|$ increases with decreasing pore cross-section,[1] i.e., $J_2 > J_1$. However, as the cross-sectional area decreases, $I_\mathrm{b,a}$ will also decrease, i.e., $I_\mathrm{b,a,1} > I_\mathrm{b,a,2}$. (b) Simulated nanopore baseline current $I_\mathrm{b,a}$ when the torus bubble bulges out by reducing its contact angle inside the 420 nm pore. For 6.3 V (pink trace), when $\theta = 69°$, $I_\mathrm{b,a} = 79.5$ μA, which agrees with experimental results [Fig. S17(c)]. (c) Rate of change of average Joule heat density in $V_\mathrm{p,c}$ [see Fig. 6(a) in the main paper], $\hat{h}_\mathrm{c} \approx \sigma|E|^2$, with contact angle $\theta$. This graph shows that for the majority of the contact angle range, the average Joule heat density inside the pore increases when the torus bubble bulges out.

**Simulation of thermal equilibrium of pore–bubble**

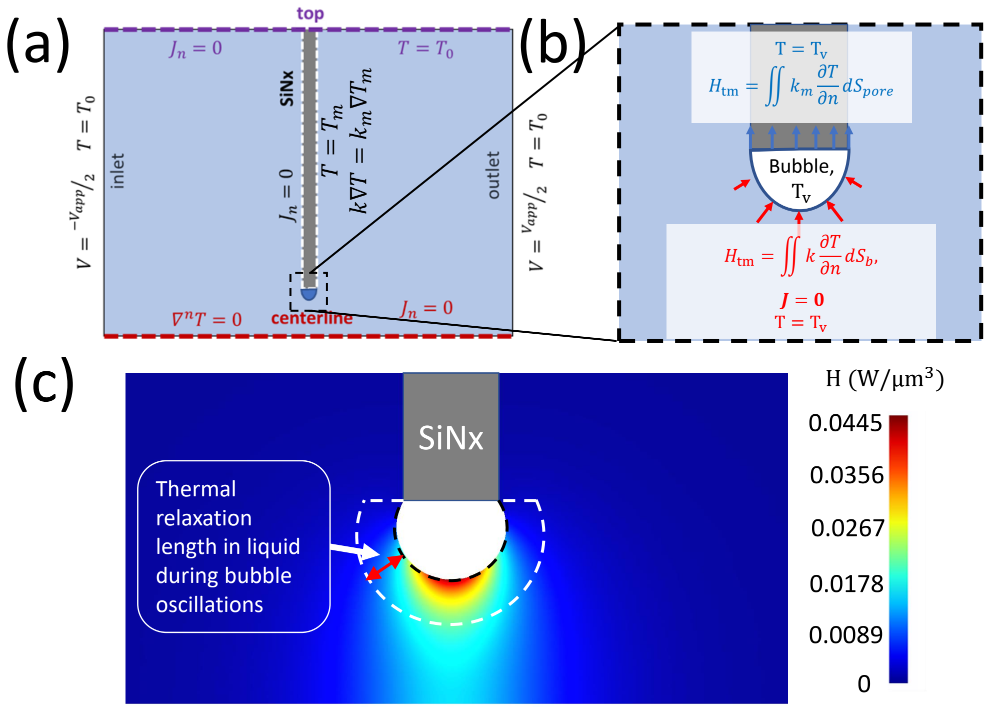


Figure S7: Nanopore–torus-bubble Joule heating model for solving the steady-state nanopore temperature distribution. (a) Axisymmetric geometry and boundary conditions applied for temperature and current.[1] (b) Boundary conditions applied on the bubble surface. The vapor inside the bubble is assumed to be in thermal equilibrium with (i) the liquid on the interface and (ii) the cylindrical silicon nitride surface on which it sits. The net heat flux from the liquid to the vapor on the liquid/vapor interface, $S_b$, is equal to the net heat flux from the vapor to the silicon nitride walls, $S_{pore}$. (c) Steady-state distribution of Joule heat density $H$ inside the nanopore.

## Simulation of torus bubble reduced mass

- Velocity potential ($\phi = \phi(r, z, \mathrm{t})$) and stream function ($\psi = \psi(r, z, \mathrm{t})$) in cylindrical co-ordinates ($r, z$) can be written as

$$u_r = \frac{\partial \phi}{\partial r} = \frac{\partial \psi}{\partial z}, \qquad u_z = \frac{\partial \phi}{\partial z} = -\frac{\partial \psi}{\partial r}$$

- Governing equation/ Continuity equation: $\frac{\partial u_r}{\partial r} + \frac{u_r}{r} + \frac{\partial u_z}{\partial z} = 0 \Rightarrow \nabla^2 \phi = 0$

- Boundary conditions, $\frac{\partial \phi}{\partial n} = 0$ is applied on Centerline, Symmetry line, SiNx wall and Far field. $n$ is the normal vector to the surface.

- Velocity boundary conditions on tracer points on bubble surface [$S_b$: $(R, Z)$] are invoked:

$$\frac{\partial \phi}{\partial n} = u_{r,b} \cdot n + u_{z,b} \cdot n$$

$$u_{r,b} = \frac{\Delta R}{\Delta t'} \text{ and } u_{z,b} = \frac{\Delta Z}{\Delta t'}$$

$\Delta R_j = \frac{R_j(\theta + \Delta\theta) - R_j(\theta)}{\Delta t'}$ where $\Delta\theta = 0.5°$. $\Delta t' = \Delta\theta / \dot{\theta}$ and $\dot{\theta}$ is contact angle velocity.

$\theta$ is the bubble contact angle and $R = R(\theta), Z = Z(\theta)$ are bubble shape co-ordinates obtained through uniform curvature torus bubble

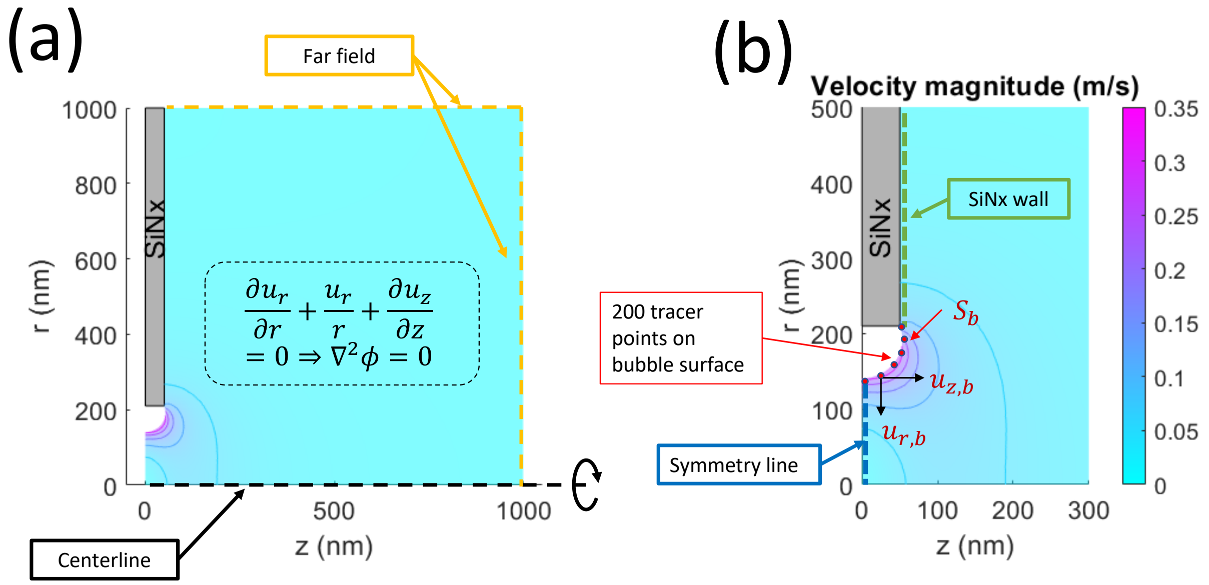


Figure S8: Geometry, boundary conditions, and governing equation for solving the potential flow equation in the nanopore fluid for pinned motion of the torus bubble: (a) axisymmetric geometry of the system; (b) zoomed view.

# S4. Boiling transition of expanded 250 nm pore

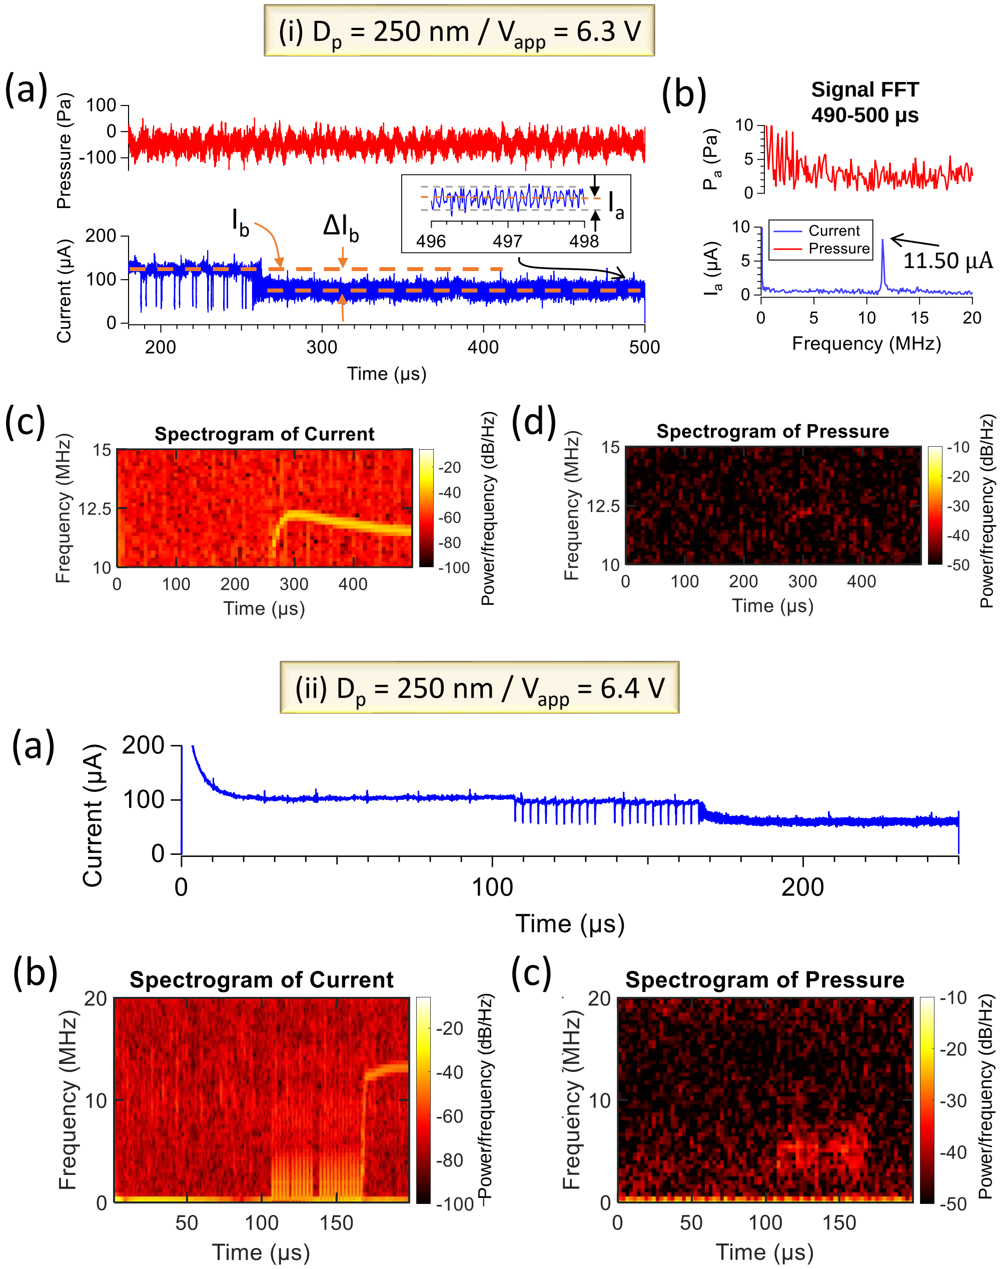


Figure S9: (i) Nucleate-to-film boiling transition at 6.3 V: (a) transient current trace; (b) fast Fourier transforms (FFTs) of current and pressure; (c) and (d) spectrograms of current and hydrophone pressure. (ii) Nucleate-to-film boiling transition at 6.4 V: (a) transient current trace; (b) and (c) spectrograms of current and hydrophone pressure.

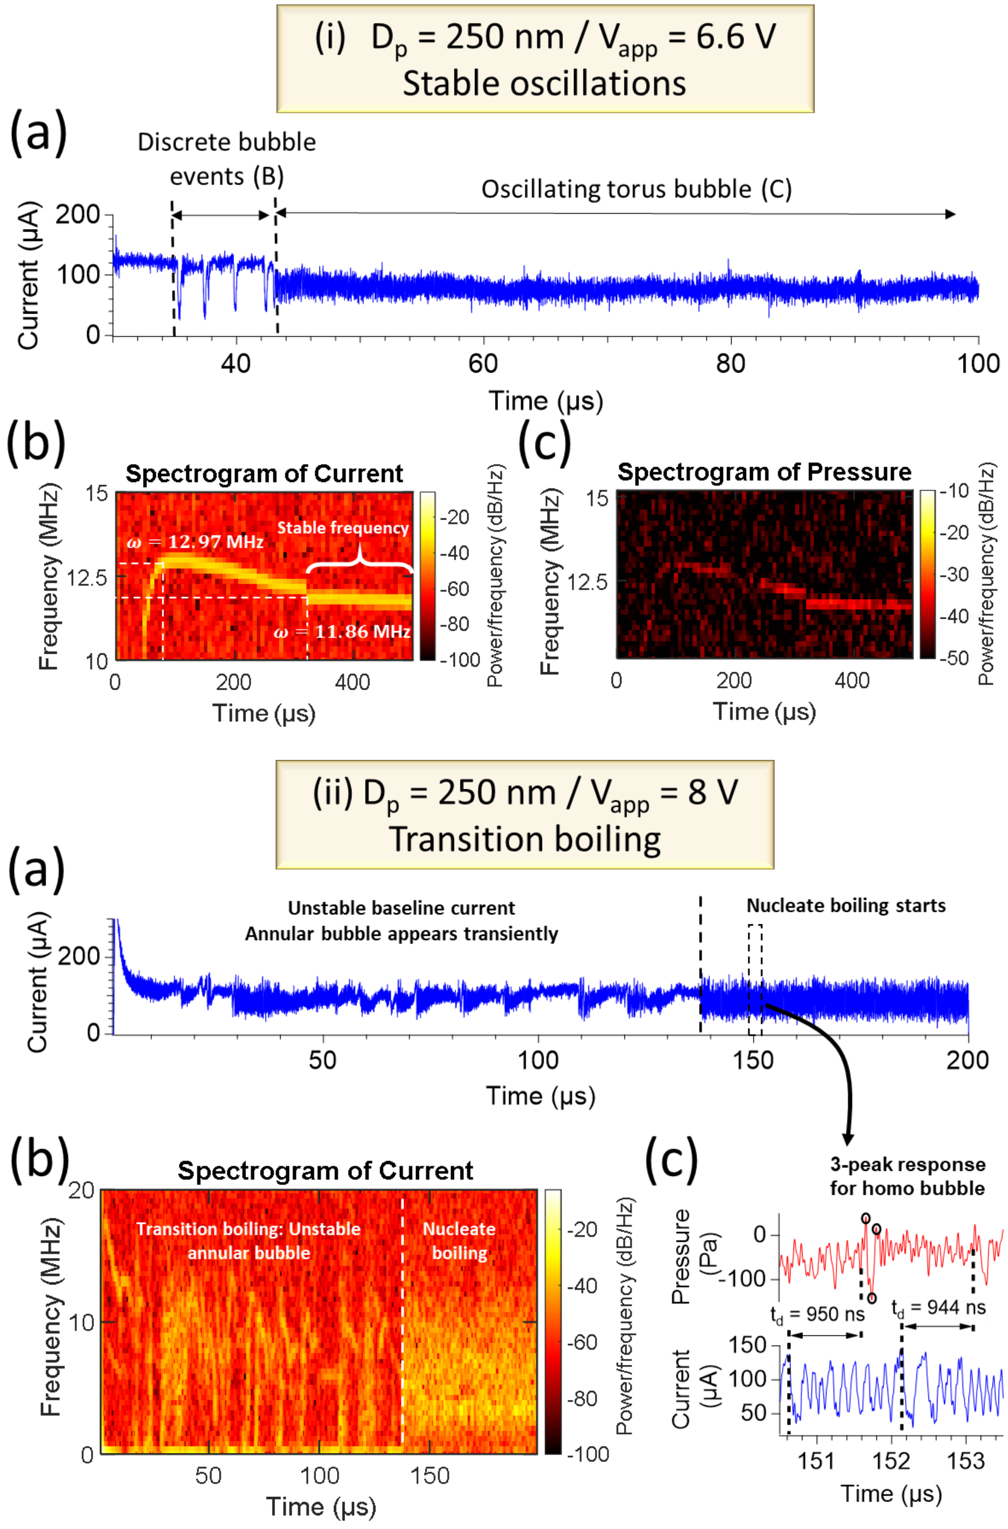


Figure S10: (i) Stable oscillatory boiling at 6.6 V: (a) transient current trace; (b) and (c) spectrograms of current and hydrophone pressure. (ii) Transition boiling at 8 V: (a) transient current trace; (b) spectrogram of current; (c) zoomed view of the current and hydrophone pressure traces in the nucleate boiling zone.

In Fig. S10(i-a), six distinct bubble nucleation events can be seen in the current trace, after each of which there is a transition to film boiling, during which oscillating current signals are seen along with baseline reduction. It should be noted that compared with the case of 6.4 V, the initial number of homogeneous bubbles decreases, demonstrating that in the low-voltage range, increasing the bias voltage (or heating rate) facilitates the transition to film boiling. Figure S10(i-b) shows that after the onset of film boiling, the frequency decreases from 12.97 MHz to 11.86 MHz over ∼250 µs. After this zone of unsteady frequency, the oscillation stabilizes at 11.86 MHz for the rest of the pulse duration. This indicates that the bubble is in thermal resonance with the Joule heating oscillations produced as a result of bubble oscillations. In other words, the temperature distribution inside the nanopore approaches a steady state. It should be noted that compared with the case of 8 V, the heating rate at 6.6 V is smaller, and thus steady-state thermal resonance is realized.

Figure S10(ii-a) shows transition boiling for a expanded 250 nmpore at 8 V. In this case, the baseline current is unstable from the onset of the pulse until ∼138 µs. During this period, the baseline current decreases intermittently for some periods of time. The current spectrogram in Fig. S10(ii-b) provides a better illustration of the underlying boiling transitions. We find that frequency bands are formed intermittently, indicating that the torus bubble forms and collapses intermittently. In between bouts of torus bubble oscillation, nucleate boiling is observed.

After ∼138 µs, the boiling permanently transitions into nucleate boiling, as evidenced by the absence of any frequency bands in the current spectrogram. Figure S10(ii-c) shows a zoomed view of the current and pressure traces during the nucleate boiling zone. We find nonuniform bubble blockage signals, with the larger blockage durations corresponding to homogeneous bubbles, as evidenced by the three distinct peak pressure responses[2] observed after constant delay times.

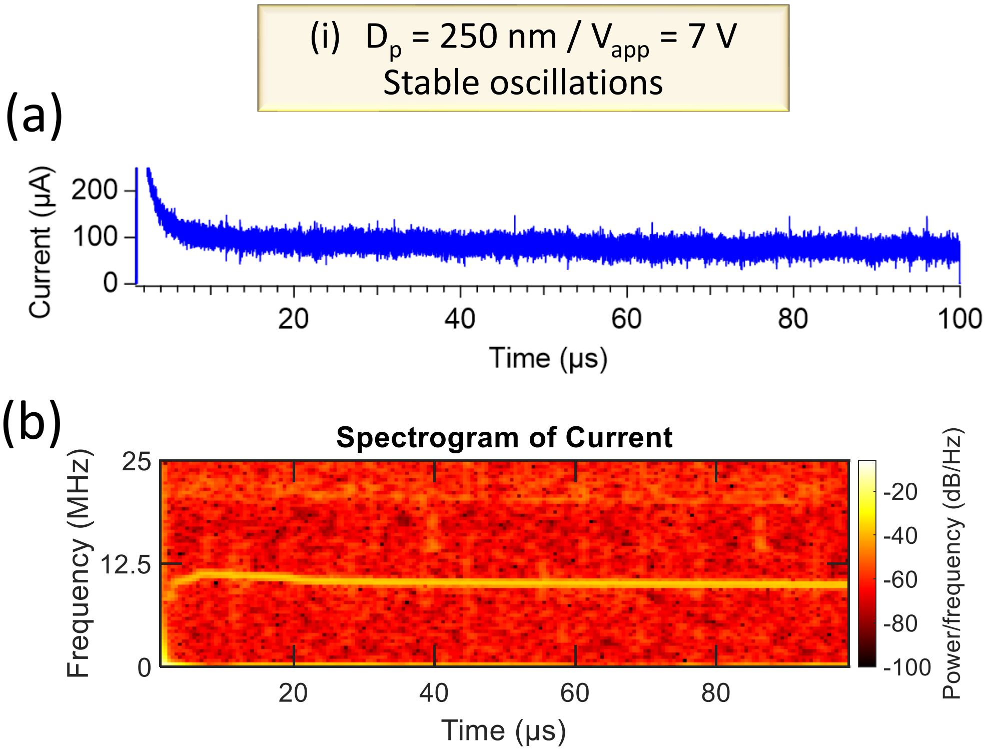


Figure S11: Stable film boiling when 7 V is applied across the expanded 250 nm pore: (a) transient current trace; (b) spectrogram of nanopore current.

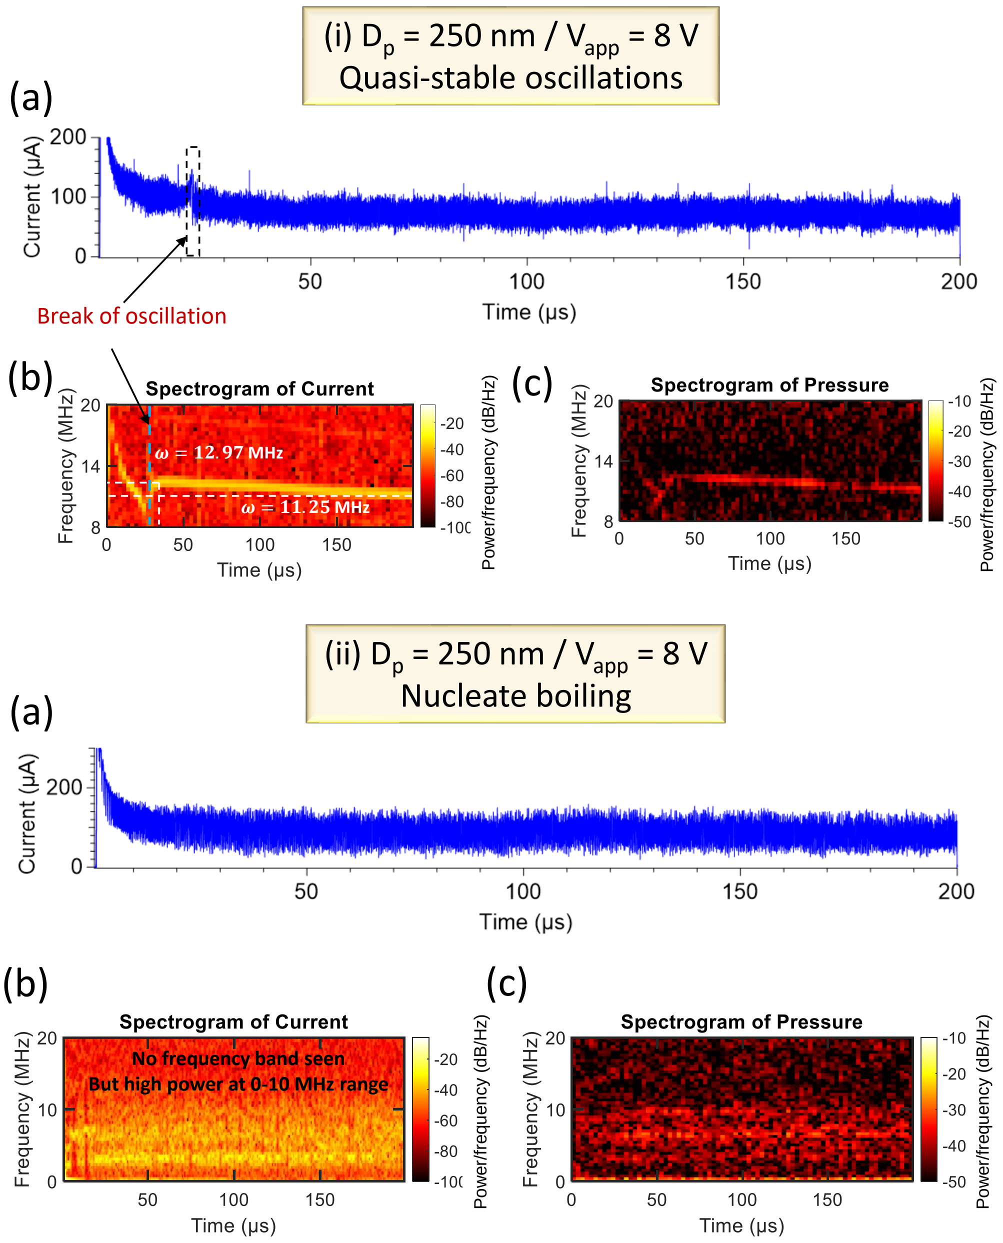


Figure S12: Two pulses of 8 V across the expanded 250 nmpore, showing two distinct boiling scenarios: (i) quasistable oscillatory boiling; (ii) nucleate boiling. (a) Transient current traces. (b) and (c) Spectrograms of current and hydrophone pressure.

In Figs. S12(i-b) and S12(i-c), distinct frequency bands are seen, signifying an oscillating torus bubble blanketing the pore surface. In Fig. S12(i-b), the frequency band for the current initially decreases rapidly, demonstrating the growth of a pinned torus bubble (explained in Fig. S13). Owing to the high rate of heating and the small torus volume, the temperature

within the unblocked nanopore volume rises unchecked, which destabilizes the torus bubble, causing it to collapse. A new torus bubble is formed and remains stable for the remainder of the pulse duration. The second torus bubble has a larger volume, which restricts the total Joule heat production inside the pore, owing to the volume exclusion effect. Thus, the second torus bubble does not destabilize. However, the frequency of the second torus bubble also decreases from 12.97 MHz at inception to 11.25 MHz at the end of the pulse. Despite the high bubble volume, due to the high voltage, the temperature within the unblocked pore volume rises slowly and never reaches a steady state, causing the bubble to expand slowly and leading to a reduction in its frequency. In Fig. S12(i-c), the frequency band for the hydrophone pressure is almost non-existent for the first torus bubble. This is because at its inception, the volume and amplitude of oscillation of the torus bubble are small. Thus, despite its higher frequency, the bubble does not create strong enough stress waves to be detected by the hydrophone above its noise level. It should be noted that the pressure of the stress waves is proportional to the bubble size and the square of the radial velocity.[2,3]

In Figs. S12(ii-b) and S12(ii-c), the spectrograms show no clear frequency bands. However, high oscillation power is noticeable in the 0–10 MHz range, indicating stochastic bubble nucleation (nucleate boiling).

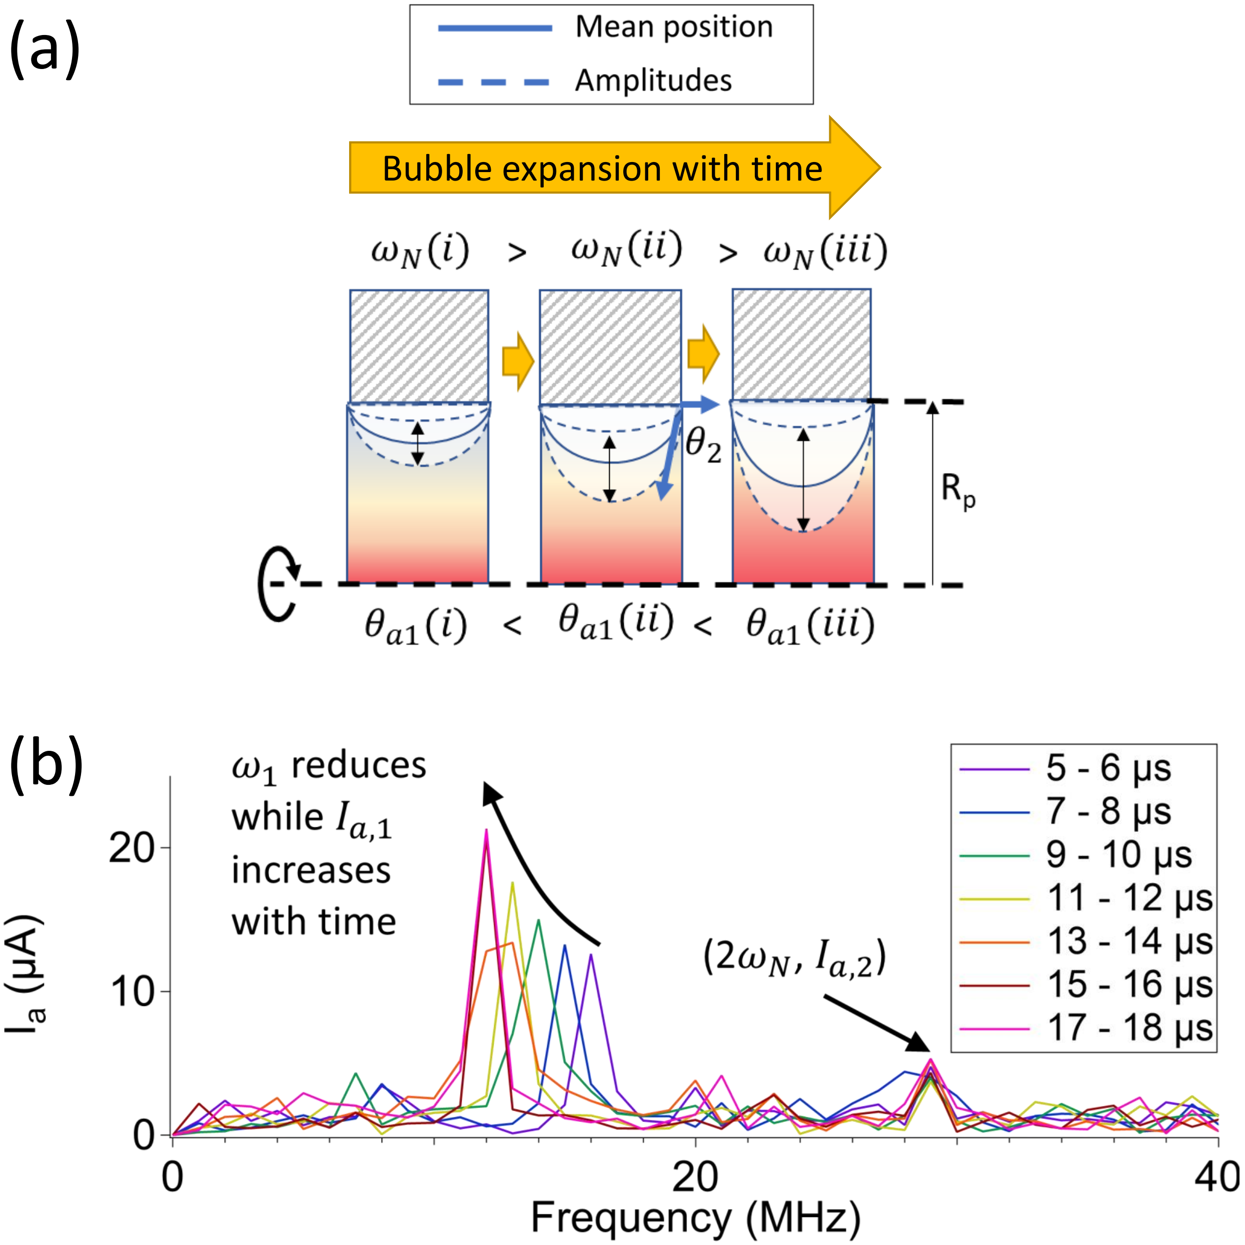


Figure S13: Explanation of early torus bubble oscillatory growth hypothesized in Fig. S12(i-a). (a) Schematic showing the pinned growth of the torus bubble at the early stage of pulsed Joule heating when the temperature distribution within the pore has not reached a steady state. Owing to the rapid rise in pore temperature, the bubble grows (the contact angle decreases). During this process, the bubble volume increases, which leads to a reduction in bubble stiffness.[4] As a result, the natural frequency of thermal self-oscillation of the torus bubble decreases, while the amplitude increases. During the early phase of heating, thermal resonance is not yet established between the nanopore Joule heating and torus bubble. Therefore, the frequency of oscillations resembles the self-oscillation frequency of the bubble. (b) FFT of the current trace taken at 1 μs intervals, showing the transient changes in bubble oscillation amplitude and frequency demonstrating pinned torus bubble growth.

## S5. Boiling transition of 340 nm pore

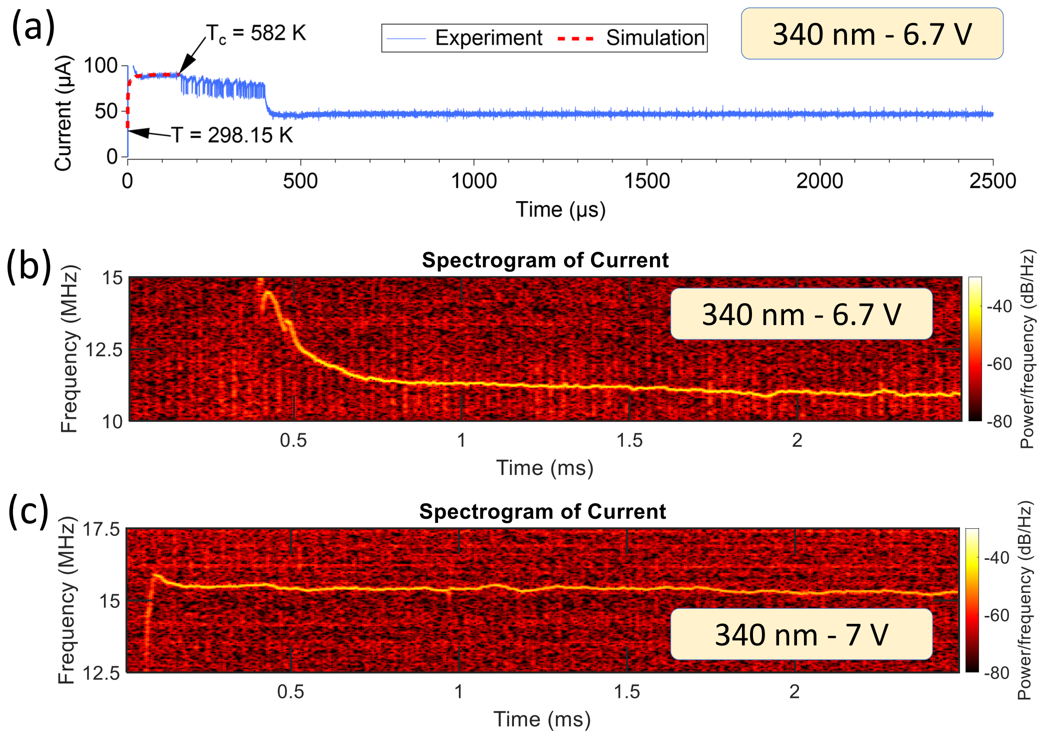


Figure S14: Boiling inside the 340-nm pore: (a) and (b) transient current trace and spectrogram at 6.7 V; (c) spectrogram at 7 V. These plots show that for smaller pores, the torus bubble frequency is higher and remains stable even at higher voltages.

## S6. Boiling transition of 460 nm pore

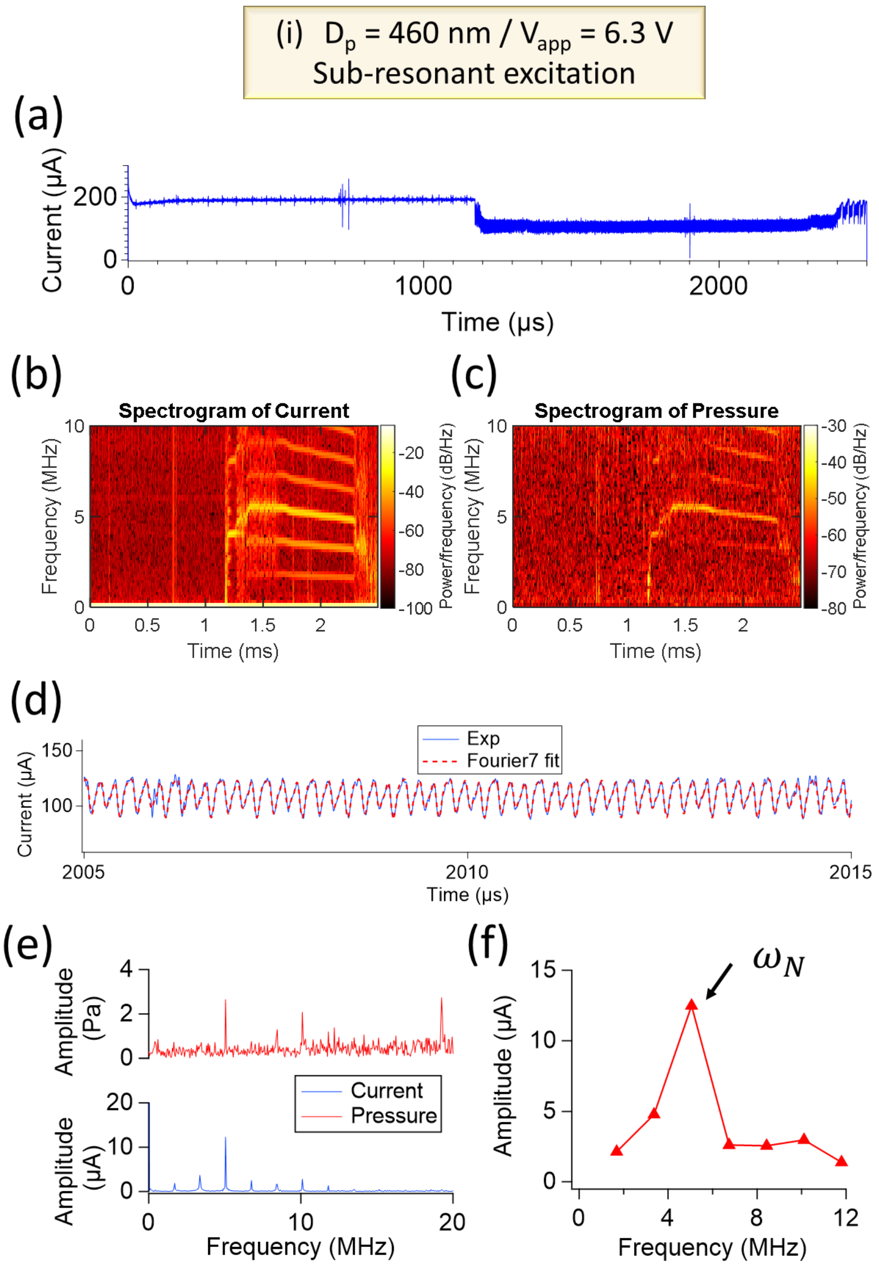


Figure S15: (a) Transient current trace. (b) and (c) Spectrograms of current and hydrophone pressure. (d) Oscillating current trace fitted with a seventh-order Fourier series. (e) FFTs of nanopore current and hydrophone pressure during the time interval from 2000 µs) to 2020 µs). Strangely, seven peaks are seen, with the highest at 4.3 MHz. (f) Amplitudes of different harmonics.

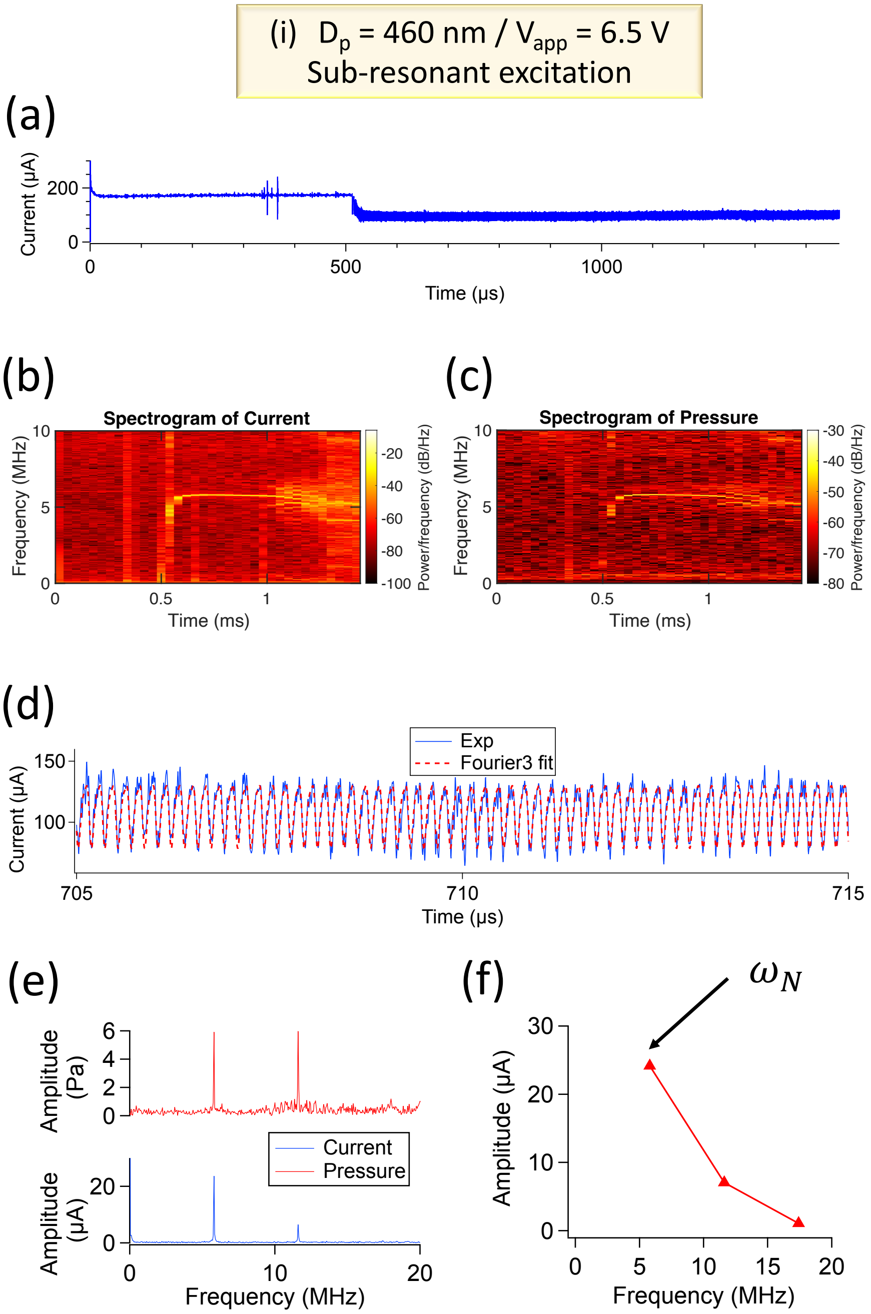


Figure S16: (a) Transient current trace. (b) and (c) Spectrograms of current and hydrophone pressure. It can be seen that the narrow frequency band representing zone C-i exists from 0.5 ms to 1 ms, before being disrupted and transitioning into zone C-ii, where the oscillations become highly nonlinear. This indicates that unlike the 340 nm pore [Fig.S14(b)], which has a stable torus bubble for several milliseconds, the 460 nm pore has a pseudostable torus bubble that is not stable in the long term. (d) Oscillating current trace fitted with a third-order Fourier series. (e) FFTs of nanopore current and hydrophone pressure during the time interval from 700 μs to 720 μs. (f) Amplitudes of different harmonics.

## S7. Boiling transition of 420 nm pore

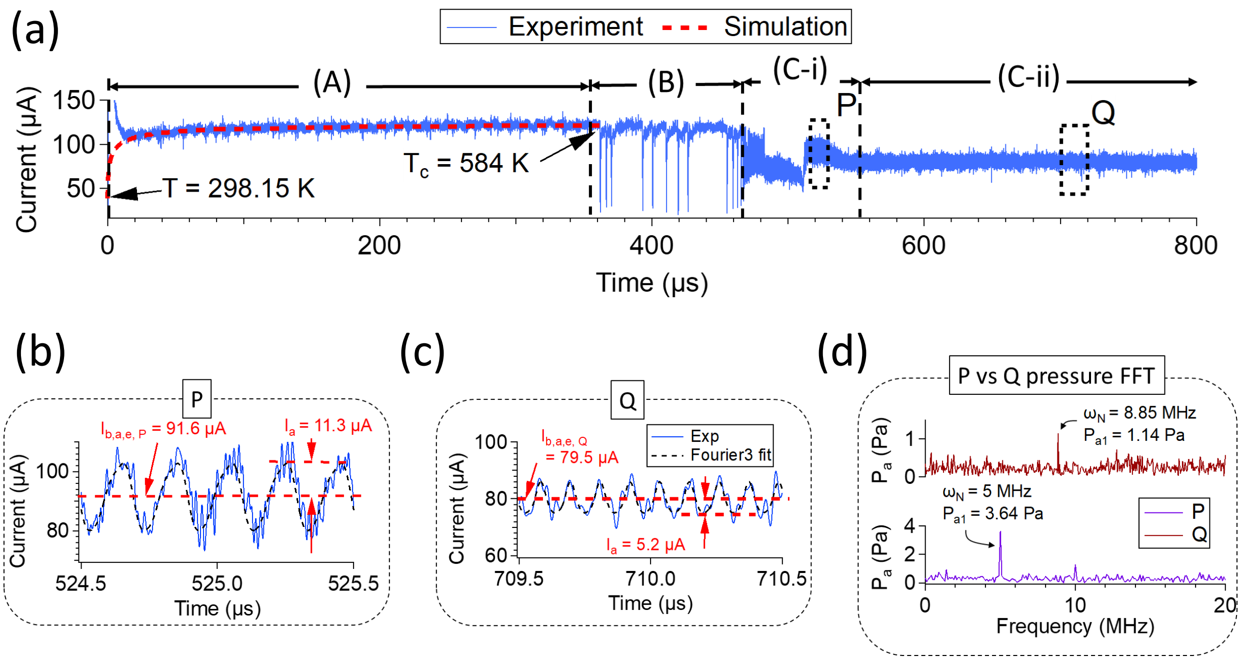


Figure S17: Boiling structure at $V_{\mathrm{app}} = 6.3$ V: (a) transient current trace; (b) oscillating current trace in zone P (unsteady film bubble); (c) oscillating current trace in zone Q (steady film bubble) fitted with a third-order Fourier series; (d) FFTs of hydrophone pressures in zones P and Q.

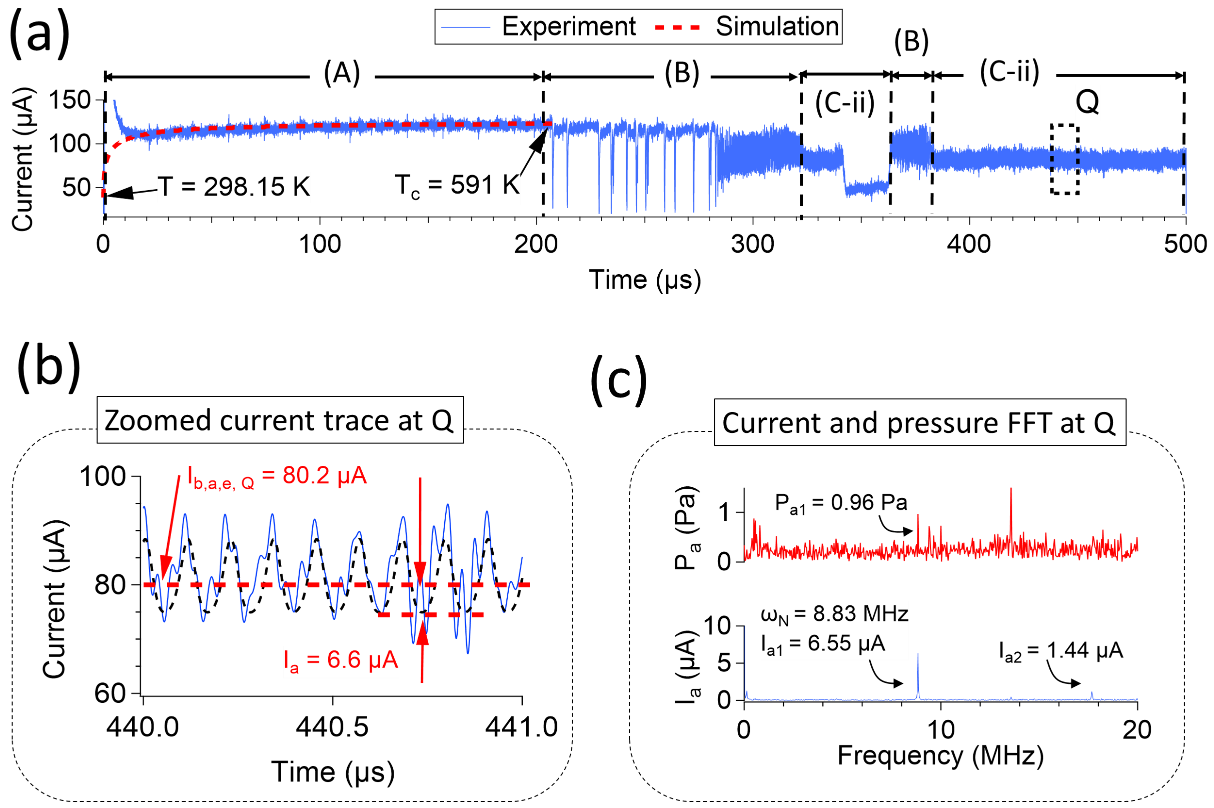


Figure S18: Boiling structure at $V_{app}$ = 6.4 V: (a) transient current trace; (b) oscillating current trace in zone Q (steady film bubble) fitted with a third-order Fourier series; (c) FFTs of nanopore current and hydrophone pressure in zone Q. It should be noted that compared with the case of 6.3 V (Fig. S17), for this experiment, the hydrophone clearance was 500 μm farther from the chip, which explains the lower pressure amplitude seen here.

# References


1. Paul, S.; Hsu, W.-L.; Magnini, M.; Mason, L. R.; Ho, Y.-L.; Matar, O. K.; Daiguji, H. Single-bubble dynamics in nanopores: Transition between homogeneous and heterogeneous nucleation. *Phys. Rev. Res.* **2020**, *2*, 043400.

2. Versluis, M.; Schmitz, B.; Von der Heydt, A.; Lohse, D. How snapping shrimp snap: Through cavitating bubbles. *Science* **2000**, *289*, 2114–2117.

3. Brennen, C. E. *Cavitation and Bubble Dynamics*; Cambridge University Press: New York, 2014.

4. Prosperetti, A. Vapor bubbles. *Annu. Rev. Fluid Mech.* **2016**, *49*, 221–248.
